# Supplementary material for: MoCL: Data-driven Molecular Fingerprint via Knowledge-aware Contrastive Learning from Molecular Graph
Source: arXiv:2106.04509 source file (2022-05-02)
Supplement: Supplementary file 1 [file appendix.tex]

% !TEX root = ./main.tex
%\textbf{}\onecolumn
\section*{Appendix}
Due to page limit, we present the additional results in this section.

\subsection*{Proof of Lemma}
\begin{lemma}
	Given two networks, the samples selected by either network can be decomposed into two subsets: agreement (A) and disagreement ($\bar{A}$) samples as compared to the other. Define $p_I=\frac{n_{\text{c}}}{n_{\text{c}}+n_{\bar{c}}}$ as the purity of a subset $I$, if $p_A > p_{\bar{A}}$, then $p_A > p_{A\cup \bar{A}}$.
\end{lemma}
\begin{proof}
\begin{align}
p_A > p_{\bar{A}}&\Leftrightarrow \frac{n_{11}}{n_{11}+n_{01}}>\frac{n_{10}}{n_{10}+n_{00}} & (\text{by definition}) \nonumber\\
&\Leftrightarrow n_{11}n_{00}> n_{10}n_{01} & (\text{simplify})  \nonumber\\
&\Leftrightarrow n_{11}(n_{00}+n_{01}) > (n_{10}+n_{11})n_{01} & (\text{add } n_{11}n_{01})\nonumber\\
&\Leftrightarrow \frac{n_{11}}{n_{01}} > \frac{n_{10}+n_{11}}{n_{00}+n_{01}} = \frac{n_{1\cdot}}{n_{0\cdot}} & (\text{re-arrange})\nonumber\\
&\Leftrightarrow \frac{1}{1+\frac{n_{01}}{n_{11}}} >  \frac{1}{1+\frac{n_{0\cdot}}{n_{1\cdot}}} &(\text{reciprocal twice})\nonumber\\
&\Leftrightarrow \frac{n_{11}}{n_{11}+n_{01}} > \frac{n_{1\cdot}}{n_{1\cdot} + n_{0\cdot}} & (\text{simplify})  \nonumber\\
&\Leftrightarrow p_A > p_{A\cup \bar{A}} & (\text{by definition}) \nonumber
\end{align}
\end{proof}

\subsection*{Additional Experimental Results} 

\begin{figure}[h!]
	\centering
	\begin{subfigure}[b]{0.18\textwidth}
		\includegraphics[width=\textwidth]{figures/noise-1.pdf}
		\caption{Symmetric 50\% noise}
	\end{subfigure}
	~ \quad \quad \quad
	\begin{subfigure}[b]{0.18\textwidth}
		\includegraphics[width=\textwidth]{figures/noise-2.pdf}
		\caption{Pairflip 45\% noise}
	\end{subfigure}
	\vspace{-1em}
	\caption{Noise examples for a 5-class problem.}\label{noise-case}
\end{figure}

Figure \ref{noise-case} shows the noise design in synthetic experiments. For symmetric flip, the label of each class is uniformly random flipped to the rest classes with equal probability. For pairflip, label of each class only flips to one different but similar class. The noise rate $\epsilon$ quantifies the overall proportion of labels that are flipped for each class. Table \ref{cnn} shows the network architecture used in synthetic experiments. Table \ref{gpu-config} shows the GPU configurations for each experiment. Table \ref{run-time} shows the run time for different number of networks. Table \ref{real-size} shows the size of unique drug profiles for each cell line with training and testing allocation. Figure \ref{nr-complete} shows the test accuracy and pure ratio under different noise rates for different methods on image data.

\begin{figure*}[tb]
	\centering
	\begin{subfigure}[b]{0.22\textwidth}
		\includegraphics[width=\textwidth]{figures/eps-10-sym-acc.pdf}
		\caption{CIFAR10 symmetric 50\%}
	\end{subfigure}
	~ \quad 
	\begin{subfigure}[b]{0.22\textwidth}
		\includegraphics[width=\textwidth]{figures/eps-10-sym-pr.pdf}
		\caption{CIFAR10 symmetric 50\%}
	\end{subfigure}
	~ \quad
	\begin{subfigure}[b]{0.22\textwidth}
		\includegraphics[width=\textwidth]{figures/eps-10-pf-acc.pdf}
		\caption{CIFAR10 pairflip 45\%}
	\end{subfigure}
	~ \quad 
	\begin{subfigure}[b]{0.22\textwidth}
		\includegraphics[width=\textwidth]{figures/eps-10-pf-pr.pdf}
		\caption{CIFAR10 pairflip 45\%}
	\end{subfigure}
	
	~ \quad 
	\begin{subfigure}[b]{0.22\textwidth}
		\includegraphics[width=\textwidth]{figures/eps-100-sym-acc.pdf}
		\caption{CIFAR100 symmetric 50\%}
	\end{subfigure}
	~ \quad 
	\begin{subfigure}[b]{0.22\textwidth}
		\includegraphics[width=\textwidth]{figures/eps-100-sym-pr.pdf}
		\caption{CIFAR100 symmetric 50\%}
	\end{subfigure}
	~ \quad 
	\begin{subfigure}[b]{0.22\textwidth}
		\includegraphics[width=\textwidth]{figures/eps-100-pf-acc.pdf}
		\caption{CIFAR100 pairflip 45\%}
	\end{subfigure}
	~ \quad 
	\begin{subfigure}[b]{0.22\textwidth}
		\includegraphics[width=\textwidth]{figures/eps-100-pf-pr.pdf}
		\caption{CIFAR100 pairflip 45\%}
	\end{subfigure}
	\vspace{-0.5em}
	\caption{Episode Curve (L: Test accuracy R: Pure ratio) w.r.t. training epochs. Each method is repeated for 5 random seeds with the variation plotted as shades. Grey lines are baseline methods and blue lines the proposed method.}\label{eps-complete}
	%\vspace{+2em}
\end{figure*}

\begin{figure*}[tb]
	\centering
	\begin{subfigure}[b]{0.22\textwidth}
		\includegraphics[width=\textwidth]{figures/bar-10-sym-acc.pdf}
		\caption{CIFAR10 symmetric 50\%}
	\end{subfigure}
	~ \quad 
	\begin{subfigure}[b]{0.22\textwidth}
		\includegraphics[width=\textwidth]{figures/bar-10-sym-pr.pdf}
		\caption{CIFAR10 symmetric 50\%}
	\end{subfigure}
	~ \quad
	\begin{subfigure}[b]{0.22\textwidth}
		\includegraphics[width=\textwidth]{figures/bar-10-pf-acc.pdf}
		\caption{CIFAR10 pairflip 45\%}
	\end{subfigure}
	~ \quad 
	\begin{subfigure}[b]{0.22\textwidth}
		\includegraphics[width=\textwidth]{figures/bar-10-pf-pr.pdf}
		\caption{CIFAR10 pairflip 45\%}
	\end{subfigure}
	
	~ \quad 
	\begin{subfigure}[b]{0.22\textwidth}
		\includegraphics[width=\textwidth]{figures/bar-100-sym-acc.pdf}
		\caption{CIFAR100 symmetric 50\%}
	\end{subfigure}
	~ \quad 
	\begin{subfigure}[b]{0.22\textwidth}
		\includegraphics[width=\textwidth]{figures/bar-100-sym-pr.pdf}
		\caption{CIFAR100 symmetric 50\%}
	\end{subfigure}
	~ \quad 
	\begin{subfigure}[b]{0.22\textwidth}
		\includegraphics[width=\textwidth]{figures/bar-100-pf-acc.pdf}
		\caption{CIFAR100 pairflip 45\%}
	\end{subfigure}
	~ \quad 
	\begin{subfigure}[b]{0.22\textwidth}
		\includegraphics[width=\textwidth]{figures/bar-100-pf-pr.pdf}
		\caption{CIFAR100 pairflip 45\%}
	\end{subfigure}
	\vspace{-0.5em}
	\caption{Final Performance (L: Test accuracy R: Pure ratio) w.r.t number of networks. Each method is repeated for 5 random seeds with error bar plotted. Grey color for baseline methods and blue color the proposed method.}\label{bar-complete}
	%\vspace{+2em}
\end{figure*}

\begin{figure*}[tb]
	\centering
	\begin{subfigure}[b]{0.22\textwidth}
		\includegraphics[width=\textwidth]{figures/nr-10-sym-acc.pdf}
		\caption{CIFAR10 symmetric 50\%}
	\end{subfigure}
	~ \quad 
	\begin{subfigure}[b]{0.22\textwidth}
		\includegraphics[width=\textwidth]{figures/nr-10-sym-pr.pdf}
		\caption{CIFAR10 symmetric 50\%}
	\end{subfigure}
	~ \quad
	\begin{subfigure}[b]{0.22\textwidth}
		\includegraphics[width=\textwidth]{figures/nr-10-pf-acc.pdf}
		\caption{CIFAR10 pairflip 45\%}
	\end{subfigure}
	~ \quad 
	\begin{subfigure}[b]{0.22\textwidth}
		\includegraphics[width=\textwidth]{figures/nr-10-pf-pr.pdf}
		\caption{CIFAR10 pairflip 45\%}
	\end{subfigure}
	
	~ \quad 
	\begin{subfigure}[b]{0.22\textwidth}
		\includegraphics[width=\textwidth]{figures/nr-100-sym-acc.pdf}
		\caption{CIFAR100 symmetric 50\%}
	\end{subfigure}
	~ \quad 
	\begin{subfigure}[b]{0.22\textwidth}
		\includegraphics[width=\textwidth]{figures/nr-100-sym-pr.pdf}
		\caption{CIFAR100 symmetric 50\%}
	\end{subfigure}
	~ \quad 
	\begin{subfigure}[b]{0.22\textwidth}
		\includegraphics[width=\textwidth]{figures/nr-100-pf-acc.pdf}
		\caption{CIFAR100 pairflip 45\%}
	\end{subfigure}
	~ \quad 
	\begin{subfigure}[b]{0.22\textwidth}
		\includegraphics[width=\textwidth]{figures/nr-100-pf-pr.pdf}
		\caption{CIFAR100 pairflip 45\%}
	\end{subfigure}
	\vspace{-0.5em}
	\caption{Performance (L: Test accuracy R: Pure ratio) w.r.t. different noise rates. Each method is repeated for 5 random seeds with the variation plotted as shades.}\label{nr-complete}
	%\vspace{+2em}
\end{figure*}

\begin{table}[b]
	\begin{tabular}{c}
		\hline
		32 $\times$ 32 RGB Image                          \\ \hline
		3 $\times$ 3 conv, 128 LReLU                      \\
		3 $\times$ 3 conv, 128 LReLU                      \\
		3 $\times$ 3 conv, 128 LReLU                      \\ \hline
		2 $\times$ 2 max-pool, stride 2, dropout $p=0.25$ \\ \hline
		3 $\times$ 3 conv, 256 LReLU                      \\
		3 $\times$ 3 conv, 256 LReLU                      \\
		3 $\times$ 3 conv, 256 LReLU                      \\ \hline
		2 $\times$ 2 max-pool, stride 2, dropout $p=0.25$ \\ \hline
		3 $\times$ 3 conv, 512 LReLU                      \\
		3 $\times$ 3 conv, 256 LReLU                      \\
		3 $\times$ 3 conv, 128 LReLU                      \\ \hline
		avg-pool                                          \\ \hline
		dense 128 $\rightarrow$ 10                        \\ \hline
	\end{tabular}
	\caption{CNN architecture used in the paper. The negative slope for each LeakyReLU is set as 0.01.}\label{cnn}
\end{table}

\begin{table}[b]
	\begin{tabular}{cccc}
		\hline
		GPU              & Data \& Noise            & CUDA & Experiment    \\ \hline
		GeForce GTX 1080 & CIFAR10 SYM 50\%  & 10.1 & Episode Curve \\
		GeForce GTX 1080 & CIFAR10 PF 45\%   & 10.1 & Episode Curve \\
		TITAN X (Pascal) & CIFAR100 SYM 50\% & 10.1 & Episode Curve \\
		TITAN X (Pascal) & CIFAR100 PF 45\%  & 10.1 & Episode Curve \\
		TITAN Xp         & CIFAR10 SYM 50\%  & 10.1 & Noise Rate    \\
		TITAN Xp         & CIFAR10 PF 45\%   & 10.1 & Noise Rate    \\
		TITAN Xp         & CIFAR100 SYM 50\% & 7.5  & Noise Rate    \\
		TITAN Xp         & CIFAR100 PF 45\%  & 7.5  & Noise Rate    \\
		Tesla M60        & Real Data        & 10.2 & All           \\ \hline
	\end{tabular}
	\caption{GPU configurations for all experiments.}\label{gpu-config}
\end{table}

\begin{table}[b]
	\begin{tabular}{ccc}
		\hline 
		Network & Time (h) &  GPU \\ \hline
		1          & 5        & 1      \\
		2          & 8        & 1      \\
		3          & 10       & 1      \\
		5          & 14       & 1      \\
		7          & 20       & 1      \\
		9          & 14       & 2      \\
		11         & 20       & 2      \\
		13         & 22       & 2      \\ \hline
	\end{tabular}
	\caption{Running time for different number of networks.}\label{run-time}
\end{table}
